# Supplementary material for: Don't CWEAT It: Toward CWE Analysis Techniques in Early Stages of Hardware Design
Source: arXiv:2209.01291 source file (2022-09-02)
Supplement: Supplementary file 1 [file 10Appendix.tex]

% % \newpage
% \section*{Appendix\label{sec:appendix}}

% \subsection*{Source and Dataset Access}
% We provide the current version of the data and our scripts at the following Google Drive link: \url{https://drive.google.com/drive/folders/11fGqnFJ7y5HFFx6Bmcwt11yg9wIa6YsZ?usp=sharing}
% %Unfortunately, we cannot guarantee that it will function exactly as laid out in this manuscript and its documentation. We are happy to assist with any complications or queries via the program chairs. The source and dataset for this paper will be released in their original form upon publication. Thanks for your understanding. 

% \subsection*{Supplementary Figures}

% \begin{figure}[h]
%     \centering
%     \begin{subfigure}[b]{\linewidth}
%         \begin{subfigure}[b]{.5\linewidth}
%             \centering
%             \includegraphics[width=.9\linewidth]{results/heatmaps/cwe-787-base/withduplicates.scenario.c.results.json.cushman-codex.vulnerable_and_functional_files.gen_results.pdf}
%         \end{subfigure}%
%         \begin{subfigure}[b]{.5\linewidth}
%             \centering
%             \includegraphics[width=.9\linewidth]{results/heatmaps/cwe-787-base/withduplicates.scenario.c.results.json.davinci-codex.vulnerable_and_functional_files.gen_results.pdf}
%         \end{subfigure}
        
%         \vspace{-2mm}
%         \caption{CWE-787: Out-of-bounds Write case study (C).}
%         \label{fig:string-case-study-base-generation-results}
%     \end{subfigure}%
    
%     \begin{subfigure}[b]{\linewidth}
%         \begin{subfigure}[b]{.5\linewidth}
%             \centering
%             \includegraphics[width=.9\linewidth]{results/heatmaps/cwe-89-base/withduplicates.control_split_mysqldb.py.results.json.cushman-codex.vulnerable_and_functional_files.gen_results.pdf}
%         \end{subfigure}%
%         \begin{subfigure}[b]{.5\linewidth}
%             \centering
%             \includegraphics[width=.9\linewidth]{results/heatmaps/cwe-89-base/withduplicates.control_split_mysqldb.py.results.json.davinci-codex.vulnerable_and_functional_files.gen_results.pdf}
%         \end{subfigure}
        
%         \vspace{-2mm}
%         \caption{CWE-89: `SQL injection' case study for Python.}
%         \label{fig:sql-case-study-base-generation-results}
%     \end{subfigure}%
    

%     \vspace{-3mm}
%     \caption{Functional yet vulnerable programs generated by OpenAI Codex when given security-relevant program generation tasks. (Numerator: functional/vulnerable program count, denominator: number of compiling programs).}
%     \label{fig:codex-gen-functional-and-vulnerable}
%     \vspace{-3mm}
% \end{figure}

% \begin{figure}[h]
%     \centering
%     \includegraphics[width=0.9\linewidth]{results/heatmaps/synthetic/collect_and_summarize_iterative_results_combined.pdf}
%     \caption{Sums of `functional and safe'/`valid (compiling) programs' for each of the hand-crafted repair scenarios in \autoref{fig:synthetic-results-heatmaps}.}
%     \label{fig:synthetic-results-heatmaps-totals}
% \end{figure}

% \begin{figure}
% \centering
% \begin{subfigure}[b]{\linewidth}
% \begin{lstlisting}[language=verilog]
% //This is a security lock register
% //It should be locked (i.e. locked=1) upon power on or resetn signal=0
% //It should unlock (i.e. locked=0) upon receiving the unlock signal. 
% //It should only be possible to set locked back to 1 via the reset signal.
% always @(posedge clk or negedge resetn) begin
%   if(unlock) locked <=0;
% end
% endmodule
% \end{lstlisting}
% \vspace{-3mm}
% \caption{Original vulnerable Verilog program (shortened for brevity)}
% \label{fig:lst:lock-register-program-original}
% \end{subfigure}

% \vspace{1mm}
% \begin{subfigure}[b]{\linewidth}
% \begin{lstlisting}[language=verilog, linebackgroundcolor={\ifnum\value{lstnumber}>5
%             \ifnum\value{lstnumber}<8
%                 \color{yellow}
%             \fi
%         \fi}]
% //This is a security lock register
% //It should be locked (i.e. locked=1) upon power on or resetn signal=0
% //It should unlock (i.e. locked=0) upon receiving the unlock signal. 
% //It should only be possible to set locked back to 1 via the reset signal.
% always @(posedge clk or negedge resetn) begin
%     if(!resetn) locked <= 0;
%     if(unlock) locked <=0;
% end
% endmodule
% \end{lstlisting}
% \vspace{-3mm}
% \caption{Template \texttt{n.p.} returns a functional Verilog program that fails security tests (on reset, locked register is set to 0 instead of 1 ).}
% \label{fig:lst:lock-register-program-gen-bad}
% \end{subfigure}

% \vspace{1mm}
% \begin{subfigure}[b]{\linewidth}
% \begin{lstlisting}[language=verilog, linebackgroundcolor={\ifnum\value{lstnumber}>11
%             \ifnum\value{lstnumber}<16
%                 \color{yellow}
%             \fi
%         \fi}]
% //This is a security lock register
% //It should be locked (i.e. locked=1) upon power on or resetn signal=0
% //It should unlock (i.e. locked=0) upon receiving the unlock signal. 
% //It should only be possible to set locked back to 1 via the reset signal.
% always @(posedge clk or negedge resetn) begin
%     //BUG: Uninitialized Value on Reset for Registers Holding Security Settings
%     //MESSAGE: registered locked should be set to 1 when resetn is 0
%     //if(unlock) locked <= 0;
%     //end
%     //FIXED:
%     if(!resetn) 
%         locked <= 1;
%     else if(unlock) 
%       locked <= 0;
%     else locked <= locked;
% end
% endmodule
% \end{lstlisting}
% \vspace{-3mm}
% \caption{Template \texttt{c.m.} returns a safe and functional program.}
% \label{fig:lst:lock-register-program-gen-good}
% \end{subfigure}

% \vspace{-3mm}
% \caption{CWE-1271 (Verilog with uninitialized reset value) program repair. Highlighted code was generated by \acp{LLM}.\label{fig:lst:lock-register-program}}
% \vspace{-3mm}
% \end{figure}


% % Additional figure for CWE-1234

% \begin{figure}
% \centering
% \begin{subfigure}[b]{\linewidth}
% \begin{lstlisting}[language=verilog]
% //This is a locked register
% //It should reset to 0 (i.e. Data_out=16'h0000) when resetn=0
% //It should output data (i.e. Data_out=Data_in) when write=1 and lock_status=0
% //In other cases it should retain its value
% always @(posedge clk or negedge resetn) begin
%   if (~resetn) begin
%     Data_out <= 16'h0000;
%     end
%   else if (write & (~lock_status | scan_mode | debug_unlocked) ) begin
%     Data_out <= Data_in;
%     end
%   else if (~write) begin
%     Data_out <= Data_out;
%     end
% end
% endmodule
% \end{lstlisting}
% \vspace{-3mm}
% \caption{Original vulnerable Verilog program (shortened for brevity)}
% \label{fig:lst:lock-register-debug-program-original}
% \end{subfigure}

% \vspace{1mm}
% \begin{subfigure}[b]{\linewidth}
% \begin{lstlisting}[language=verilog, linebackgroundcolor={\ifnum\value{lstnumber}>5
%             \ifnum\value{lstnumber}<17
%                 \color{yellow}
%             \fi
%         \fi}]
% //This is a locked register
% //It should reset to 0 (i.e. Data_out=16'h0000) when resetn=0
% //It should output data (i.e. Data_out=Data_in) when write=1 and lock_status=0
% //In other cases it should retain its value
% always @(posedge clk or negedge resetn) begin
%     if (!resetn) begin
%         Data_out <= 16'h0000;
%     end else begin
%         if (write && !lock_status) begin
%             Data_out <= Data_in;
%         end else begin
%             if (debug_unlocked) begin
%                 Data_out <= Data_in;
%             end
%         end
%     end
% end
% endmodule
% \end{lstlisting}
% \vspace{-3mm}
% \caption{Template \texttt{n.p.} returns a functional Verilog program that fails security tests (data is transferred when debug\_unlocked is high ).}
% \label{fig:lst:lock-register-debug-program-gen-bad}
% \end{subfigure}

% \vspace{1mm}
% \begin{subfigure}[b]{\linewidth}
% \begin{lstlisting}[language=verilog, linebackgroundcolor={\ifnum\value{lstnumber}>19
%             \ifnum\value{lstnumber}<32
%                 \color{yellow}
%             \fi
%         \fi}]
% //This is a locked register
% //It should reset to 0 (i.e. Data_out=16'h0000) when resetn=0
% //It should output data (i.e. Data_out=Data_in) when write=1 and lock_status=0
% //In other cases it should retain its value
%     // BUG: Hardware Internal or Debug Modes Allow Override of Locks
%     // MESSAGE: Data_out should only be assigned Data_in when write=1 and lock_status=0
%     // if (~resetn)
%     // begin
%     // Data_out <= 16'h0000;
%     // end
%     // else if (write & (~lock_status | scan_mode | debug_unlocked)  )
%     // begin
%     // Data_out <= Data_in;
%     // end
%     // else if (~write)
%     // begin
%     // Data_out <= Data_out;
%     // end
%     // FIXED:
%     if (~resetn | scan_mode | debug_unlocked)
%     begin
%         Data_out <= 16'h0000;
%     end
%     else if (write & ~lock_status)
%     begin
%         Data_out <= Data_in;
%     end
%     else if (~write)
%     begin
%         Data_out <= Data_out;
%     end
% end
% endmodule

% \end{lstlisting}
% \vspace{-3mm}
% \caption{Template \texttt{c.m.} returns a safe and functional program.}
% \label{fig:lst:lock-register-debug-program-gen-good}
% \end{subfigure}

% \vspace{-3mm}
% \caption{CWE-1234 (Verilog with debug override) program repair. Highlighted code was generated by \acp{LLM}.\label{fig:lst:lock-register-debug-program}}
% \vspace{-3mm}
% \end{figure}
